# Supplementary material for: Topological flat bands in hyperbolic lattices
Source: arXiv:2408.16615 source file (2024-08-29)
Supplement: Supplementary file 1 [file SM.pdf]

# Supplemental material for "Toplogical flat bands in hyperbolic lattices"

Dong-Hao Guan,[1,2] Lu Qi,[2] Yuan Zhou,[1,*] Ai-Lei He,[2,†] and Yi-Fei Wang[3,4]

[1]*National Laboratory of Solid State Microstructures and Department of Physics, Nanjing University, Nanjing 210093, China*
[2]*College of Physics Science and Technology, Yangzhou University, Yangzhou 225002, China*
[3]*Zhejiang Institute of Photoelectronics & Zhejiang Institute for Advanced Light Source, Zhejiang Normal University, Jinhua 321004, China*
[4]*Center for Statistical and Theoretical Condensed Matter Physics, and Department of Physics, Zhejiang Normal University, Jinhua 321004, China*

In main text, we systematically investigated topological flat bands (TFBs) in hyperbolic analogs of kagome lattices. Based on the Abelian hyperbolic band theory, we found that flatness ratios of the present hyperbolic TFB models are more than 15. This supplemental material contains: 1. TFBs in two-dimensional (2D) Euclidean kagome lattice; 2. The Chern number matrix of each hyperbolic TFBs; 3. TFBs of hyperbolic kagome model with open boundary conditions; 4. Numbers of mixing subbands of hyperbolic TFBs.

## S1. TFBS IN 2D EUCLIDEAN KAGOME LATTICE

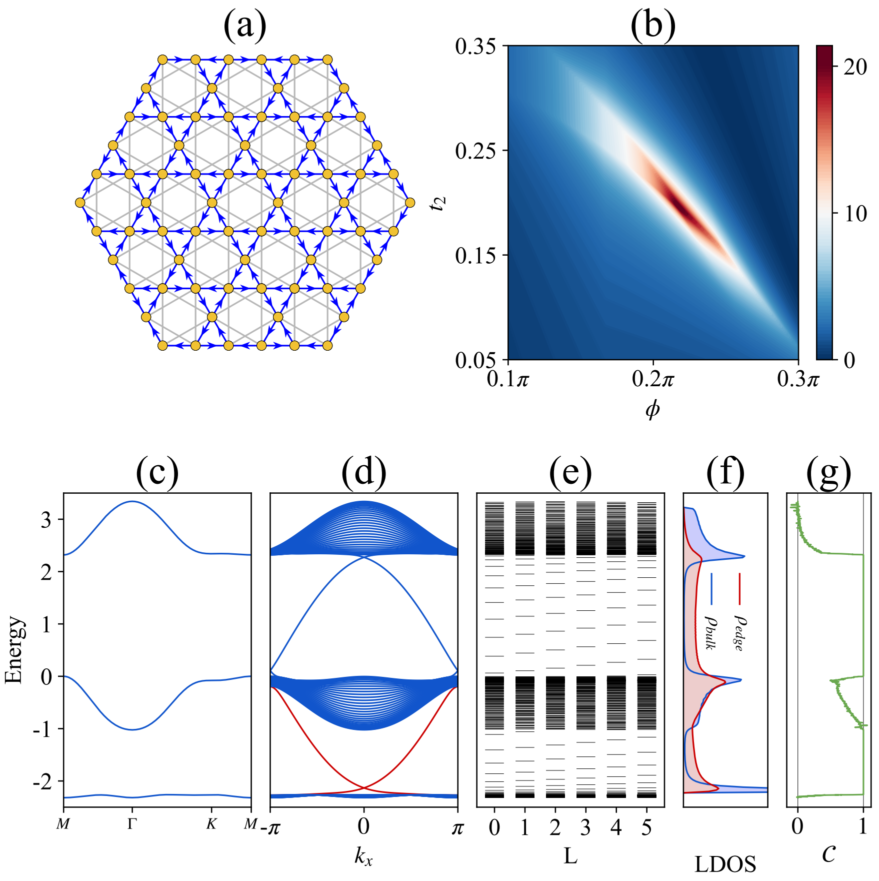


FIG. 1: (color online). (a) Lattice structure of 2D Euclidean kagome lattice with with near-neighbor (NN) along blue bonds and next-near-neighbor (NNN) along gray bonds hoppings. The staggered magnetic fluxes are added along the arrows. (b) Color map of the flatness ratio as a function of the NNN hopping potential $t_2$ and phase factor $\phi$. (c) Bulk energy bands along the high symmetric points Γ, $M$ and $K$ with the TFB parameter. (d) The corresponding energy bands on cylinder geometry which $x$ direction is with periodic boundary condition and $y$ direction with open boundary condition. (e) Energy spectrum with the TFB parameter in disk geometry with sixfold rotational symmetry. (f) The edge and bulk local density of state ($\rho_{edge}$ and $\rho_{bulk}$) of kagome TFB model in disk geometry. (g) The real-space Chern number $\mathcal{C}$ as a function of energy. Here, we consider a 2550-site kagome disk.

TFBs of 2D Euclidean kagome model [lattice structure shown in Fig. 1 (a)] has been proposed in Ref. [1]. When the hopping parameters are $t_1 = -1.0$, $t_2 = 0.19$ and $\phi = 0.22\pi$, the flatness ratio of the lowest band is about 20 [details in Fig. 1 (b) and the corresponding bulk and edge bands in Fig. 1 (c)-(d)]. When we consider the kagome TFB model in a disk geometry with sixfold rotational symmetry, one can obtain the energy spectrum arranged by angular momentum $L$ [see Fig. 1 (e)]. To characterize features of this energy spectrum, the bulk and edge local density of state (LDOS) and real-space Chern number are present in Fig. 1 (f) and (g). We find the lowest band with narrow band and non-zero Chern number in terms of the LDOS and real-space Chern number, which reveals the existence of the TFB. Here, we calculate the real-space Chern number using Kitaev formula [2], which is defined as,

$$\mathcal{C} = 12\pi i \sum_{j\in A}\sum_{k\in B}\sum_{l\in C}\left(P_{jk}P_{kl}P_{lj} - P_{jl}P_{lk}P_{kj}\right), \tag{1}$$

where, $j$, $k$, $l$ respectively denote the vertex in A, B and C regions arranged in the clockwise order [2]. $P_{jk}$ is the matrix element of projector operator $\hat{P}$, defined as $P_{jk} = \sum_{E_n<E} \Psi_n(j)\Psi_n^*(k)$. The real-space Chern number is closely related to the chosen fermi energy $E$ and as shown in Fig. 1 (g), a substantial plateau with a quantized real-space Chern number emerges, well consisting with the edge states colored with red in Fig. 1 (d).

## S2. CHERN NUMBER MATRIX

Based on the crystallography of hyperbolic lattices [3], these hyperbolic lattice models host more than two translational directions and their corresponding Brillouin zones more than 2D. To character their topological properties, we use Chern number matrix where each element $\mathcal{C}_{ij}$ denotes the Chern number calculated in a 2D $k$-space (the corresponding momenta $k_i$ and $k_j$) and other momenta are set zero. The Chern number $\mathcal{C}_{ij}$ along $k_i$ and $k_j$ is defined as,

$$\mathcal{C}_{ij}\left(\varepsilon_F\right) = \sum_{\varepsilon_\alpha<\varepsilon_F} \frac{1}{2\pi}\int_{BZ} \mathcal{F}^{\alpha}\left(k_i, k_j\right) \mathrm{d}k_i \mathrm{d}k_j. \tag{2}$$

Here, $\mathcal{F}^{\alpha}(k_i, k_j)$ indicates the berry curvature of the $\alpha$th band. On account of several bands mixing together in the lowest flat bands, $\mathcal{F}(k_i, k_j)$ of all flat bands is calculated together.

Based on the definition of Chern number [see Eq. (2)], one can easily obtain the $\mathcal{C}_{ij}$ of lowest flat bands for each hyperbolic lattice. As a consequence, we can summarize all the results using a Chern number matrix, *i.e.*,

$$\mathcal{C}_{HKG} = \begin{pmatrix} 0 & +1 & -1 & +1 & -1 & +1 \\ -1 & 0 & +1 & -1 & +1 & -1 \\ +1 & -1 & 0 & +1 & -1 & +1 \\ -1 & +1 & -1 & 0 & +1 & -1 \\ +1 & -1 & +1 & -1 & 0 & +1 \\ -1 & +1 & -1 & +1 & -1 & 0 \end{pmatrix}, \tag{3}$$

$$\mathcal{C}_{OKG} = \begin{pmatrix} 0 & +1 & -1 & +1 \\ -1 & 0 & +1 & -1 \\ +1 & -1 & 0 & +1 \\ -1 & +1 & -1 & 0 \end{pmatrix}, \tag{4}$$

$$\mathcal{C}_{NKG} = \begin{pmatrix} 0 & -1 & +1 & -1 & +1 & -1 & +1 & -1 \\ +1 & 0 & -1 & +1 & -1 & +1 & -1 & +1 \\ -1 & +1 & 0 & -1 & +1 & -1 & +1 & -1 \\ +1 & -1 & +1 & 0 & -1 & +1 & -1 & +1 \\ -1 & +1 & -1 & +1 & 0 & -1 & +1 & -1 \\ +1 & -1 & +1 & -1 & +1 & 0 & -1 & +1 \\ -1 & +1 & -1 & +1 & -1 & 1 & 0 & -1 \\ +1 & -1 & +1 & -1 & +1 & -1 & +1 & 0 \end{pmatrix}, \tag{5}$$

and

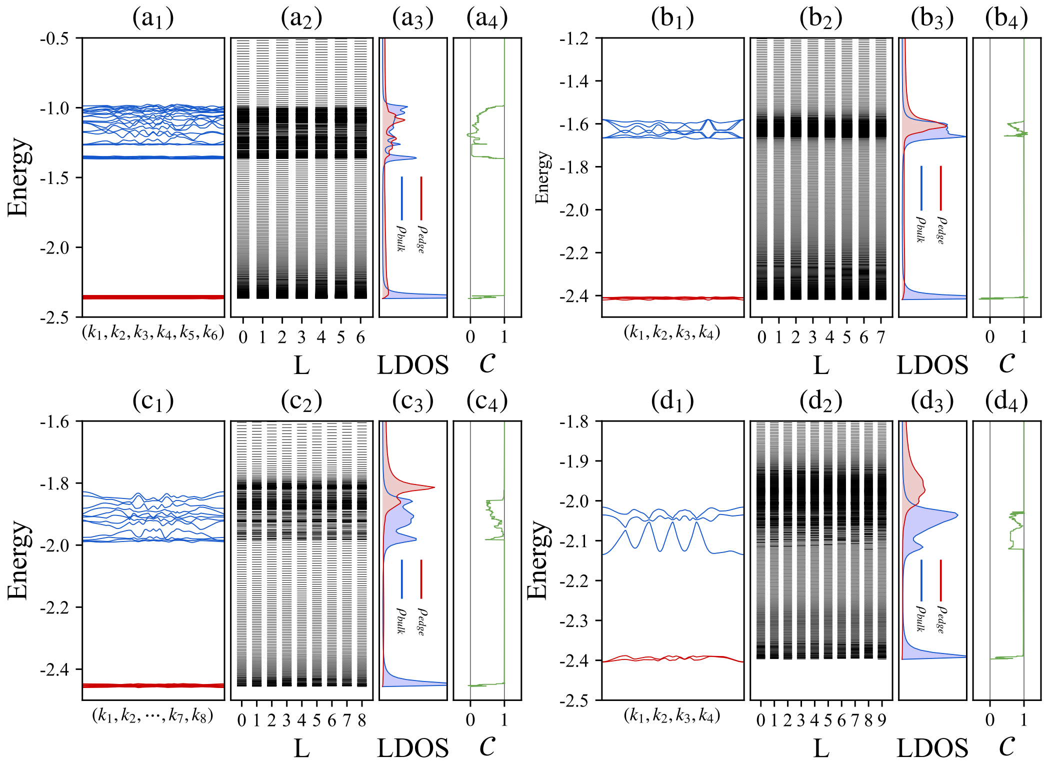


FIG. 2: (color online). Energy bands, local density of state (LDOS) and local Chern numbers of (a) heptagon-kagome (HKG), (b) octagon-kagome(OKG), (c)the nonagon-kagome (NKG) and (d) decagon-kagome (DKG) lattices. Here, we present the bulk ($\rho_{bulk}$) and edge ($\rho_{edge}$) LDOS, respectively. Here, we consider 7511-site HKG, 13080-site OKG, 8874-site NKG and 19270-site DKG, respectively.

$$\mathcal{C}_{DKG} = \begin{pmatrix} 0 & -1 & +1 & -1 \\ +1 & 0 & -1 & +1 \\ -1 & +1 & 0 & -1 \\ +1 & -1 & +1 & 0 \end{pmatrix}. \tag{6}$$

Here, we set $\mathcal{C}_{ii} = 0$, because there is not well-defined for Chern number in one dimension.

## S3. TFBS OF HYPERBOLIC KAGOME MODELS WITH OPEN BOUNDARY CONDITIONS

In this section, we choose finite hyperbolic kagome models with open boundary conditions and calculate their corresponding TFBs (see Fig. 2). To identify these TFBs, we also present the bulk and edge local density of state and local Chern number in Fig. 2. We find that TFBs with periodic boundary conditions are almost fully consistent with the ones with open boundary conditions. Here, we adopt the best TFB parameters which are $t_2 = 0.188, \phi = 0.215\pi$ for HKG model, $t_2 = 0.185, \phi = 0.210\pi$ for OKG model, $t_2 = 0.183, \phi = 0.206\pi$ for NKG model, and $t_2 = 0.146, \phi = 0.232\pi$ for DKG model.

On account of the existence of non-Abelian translation in hyperbolic lattices, non-Abelian hyperbolic band theory are required, instead of Abelian hyperbolic band theory. To approximate the hermodynamic limit commonly requires the systems with infinite sites. Continued-fraction method [4–6] can only obtain the the LDOS of hyperbolic kagome models with a large mount of atoms. The diagonal matrix elements of the Green's function $[G(E)]_{nn} = \langle n|G(E)|n\rangle$

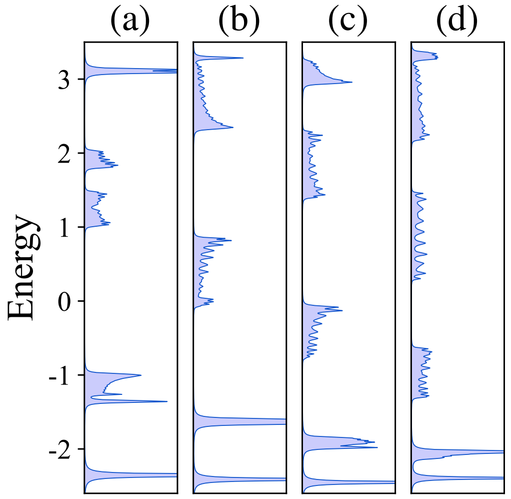


FIG. 3: (color online). Local density of state (LDOS) of (a) heptagon-kagome, (b) octagon-kagome, (c)the nonagon-kagome and (d) decagon-kagome lattices. Here, the size of each hyperbolic kagome lattice is more than $10^8$.

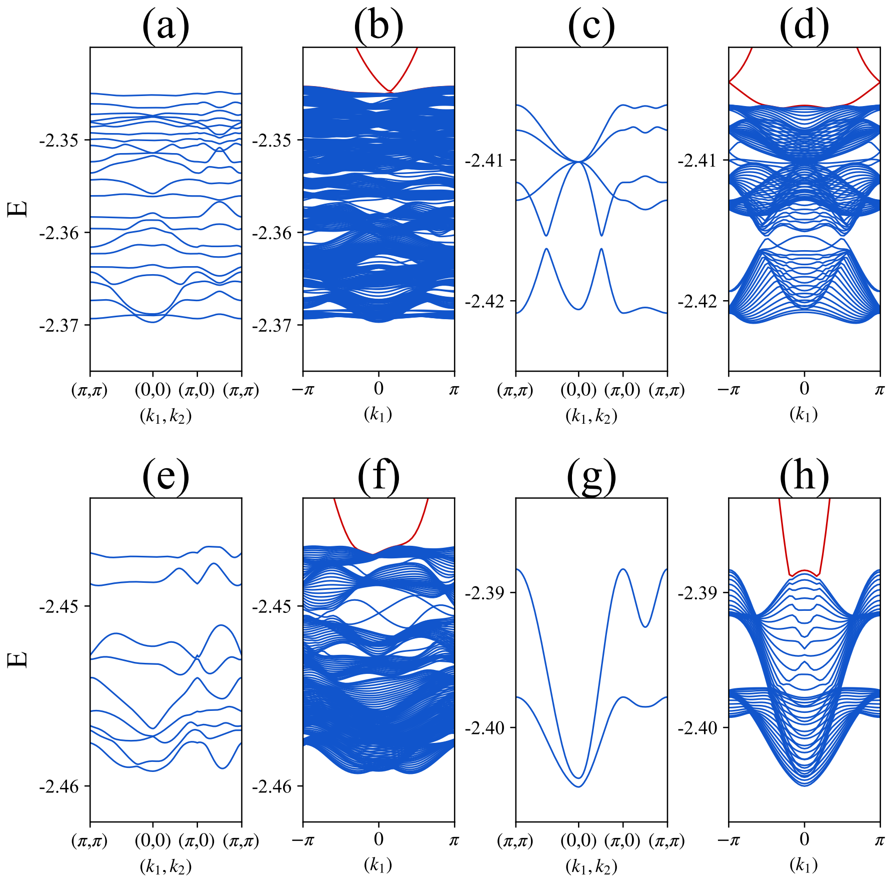


FIG. 4: (color online). TFBs of (a)-(b) HKG, (c)-(d) OKG, (e)-(f) NKG and (g)-(h) DKG lattice models. Here, we present the bulk energy bands along ($k_1$,$k_2$)= ($\pi$, $\pi$), (0, 0), ($\pi$, 0) and ($\pi$, $\pi$) in (a), (c), (e) and (g). The bulk and edge bands are shown in (b), (d), (f) and (h) with periodic boundary along $k_1$ direction and open boundary along $k_2$ direction. Here, other momenta $k_i$ are set zero.

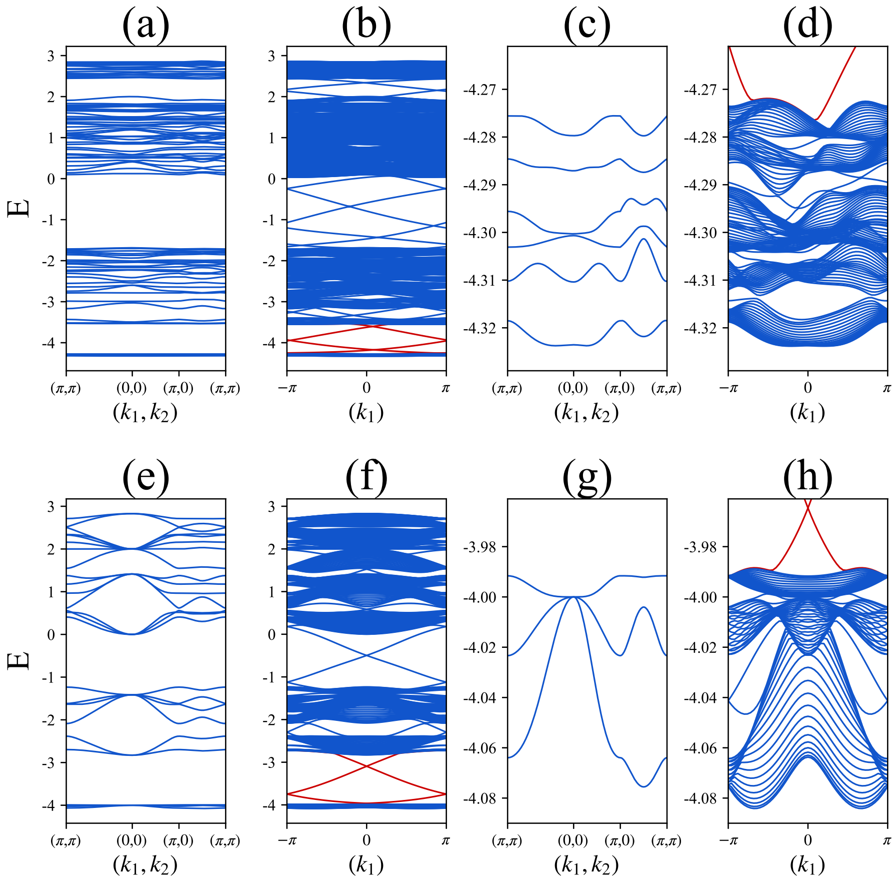


FIG. 5: (color online). TFBs of (a)-(d) HKG and (e)-(h) OKG lattice models. Here, we present the bulk energy bands along ($k_1$,$k_2$)= ($\pi$, $\pi$), (0, 0), ($\pi$, 0) and ($\pi$, $\pi$) in (a), (c), (e) and (g). The bulk and edge bands are shown in (b), (d), (f) and (h) with periodic boundary along $k_1$ direction and open boundary along $k_2$ direction. Here, other momenta $k_i$ are set zero.

($G(E) = 1/(E - H)$) can be expanded as [4–6],

$$[G(E)]_{nn} = \cfrac{1}{E - a_1 - \cfrac{b_1}{E - a_2 - \cfrac{b_2}{E - a_3 - \cfrac{b_3}{\cdots}}}}, \tag{7}$$

where the coefficients $(a_n, b_n)$ are rational numbers which depend on the state $|n\rangle$. These coefficients are directly related to those computed via the recursion method [4, 5]. The LDOS can be obtained by,

$$\rho_n(E) = -\frac{1}{\pi} \lim_{\varepsilon \to 0^+} \mathrm{Im}[G(E + \mathrm{i}\,\varepsilon)]_{nn}, \tag{8}$$

Based on this method, we consider several hyperbolic kagome models with more than $10^8$ sites and obtain the bulk LDOS (details in Fig. 3). Referring to Fig. 4, we find the bulk LDOS for hyperbolic kagome models in a finite disk is in accord with the one obtained by the continued-fraction method, which reveals the robustness of these TFBs.

## S4. NUMBERS OF LOW-ENERGY SUBBANDS IN HYPERBOLIC TFBS

In the main text, we find that there are several subbands mixing together in hyperbolic TFBs, instead of single flat band in 2D Euclidean kagome lattice [see Fig. 1 (c)]. Various numbers of low-energy subbands in these hyperbolic TFBs. There are respectively 22, 5, 9 and 2 subbands in the TFBs of HKG, OKG, NKG and DKG models (see Fig. 4). We present the TFBs of HKG model with other hopping parameters which are given in Ref. [7] [details in

Fig. 5 (a)-(d)]. We find that the flatness ratio is about 18 and there are six subbands mixing together [details in Fig. 5 (c) and (d)]. We also calculate the hyperbolic band which has studied in Ref. [7] and find that there are three subbands mixing together with flatness ratio about 13 [details in Fig. 5 (e)-(h)].

* Electronic address: zhouyuan@nju.edu.cn
† Electronic address: heailei@yzu.edu.cn

[1] R. Liu, W.-C. Chen, Y.-F. Wang, and C.-D. Gong, Journal of Physics: Condensed Matter **24**, 305602 (2012), URL https://doi.org/10.1088/0953-8984/24/30/305602.
[2] A. Kitaev, Annals of Physics **321**, 2 (2006), ISSN 0003-4916, january Special Issue, URL https://www.sciencedirect.com/science/article/pii/S0003491605002381.
[3] I. Boettcher, A. V. Gorshkov, A. J. Kollár, J. Maciejko, S. Rayan, and R. Thomale, Phys. Rev. B **105**, 125118 (2022), URL https://link.aps.org/doi/10.1103/PhysRevB.105.125118.
[4] R. Haydock, V. Heine, and M. J. Kelly, Journal of Physics C: Solid State Physics **5**, 2845 (1972), URL https://dx.doi.org/10.1088/0022-3719/5/20/004.
[5] R. Haydock, V. Heine, and M. J. Kelly, Journal of Physics C: Solid State Physics **8**, 2591 (1975), URL https://dx.doi.org/10.1088/0022-3719/8/16/011.
[6] R. Mosseri and J. Vidal, Phys. Rev. B **108**, 035154 (2023), URL https://link.aps.org/doi/10.1103/PhysRevB.108.035154.
[7] H. Yuan, W. Zhang, Q. Pei, and X. Zhang, Phys. Rev. B **109**, L041109 (2024), URL https://link.aps.org/doi/10.1103/PhysRevB.109.L041109.
